# Supplementary material for: Gating Dropout: Communication-efficient Regularization for Sparsely Activated Transformers
Source: arXiv:2205.14336 source file (2022-07-04)
Supplement: Supplementary file 1 [file appendix.tex]

\subsection{Effect of Number of Experts}
We investigate the effect of the number of experts on the throughput for \extension{} on the WMT-10 dataset.
We only report results for \extension{} for the same reason from the previous subsection.
%In Table~\ref{table:ablation_expert_num}, we report the results 
We have run experiments for \extension{} with three different values for the number of experts: $32$, $64$ and $128$.
%For the purpose of comparison, the results of the baseline is also included.
Note that we always use $16$ V100 GPUs for these experiments.
We observe that the throughput is almost stable when the number of experts changes, because the number of GPUs is constant.
As we increase the number of experts, we can see that the BLEU scores at convergence keeps improving (i.e., $24.92$, $24.95$ and $25.12$ for $32$, $64$ and $128$ experts, respectively).
Similar trend has been observed in the baseline MoE models~\cite{kim2021scalable}.
Our results imply that when applying \method{} during MoE model training, this nice trend is preserved.
